# Supplementary material for: Privacy-preserving Chunk Scheduling in a BitTorrent Implementation of Federated Learning
Source: arXiv:2605.10499 source file (2026-05-14)
Supplement: Supplementary file 1 [file Appendix_1.tex]

\section{NP-Completeness of the Chunk Scheduling Problem in \emph{FLTorrent}}

We establish NP-completeness by formulating the decision version of the Chunk Scheduling Problem (CSP), arguing that it lies in NP, and proving NP-hardness via polynomial reductions from the classical scheduling problem \(P\mid\text{prec}\mid C_{\max}\) and from \textsc{3-Partition}. The former is a canonical precedence-constrained identical-machines makespan problem known to be NP-hard (see, e.g., \cite{Ullman1975}), while \textsc{3-Partition} is strongly NP-complete \cite{GareyJohnson1979}; together these imply NP-hardness and, in fact, strong NP-hardness of CSP under standard encodings.

\subsection{Chunk Scheduling Problem (Decision Version)}
We consider a round-limited scheduling model that captures \emph{FLTorrent}'s warm-up dissemination. Let the peer connectivity be a graph \(G_P=(V_P,E_P)\) with per-peer bandwidth capacities \(c_P:V_P\!\to\!\mathbb{R}_{>0}\). For each data chunk \(c\in C\) initially residing at a designated producer \(s(c)\in V_P\) and required by a designated consumer \(t(c)\in V_P\), the chunk transmission graph \(G_C=(V_C,E_C)\) encodes which transfers are possible and (optionally) which transfers must precede others before a given transfer may start. A schedule chooses, for each chunk \(c\), a (here: direct) peer-to-peer transmission \((u,v)\in E_P\) that realizes \(s(c)\!\to\!t(c)\)\,, and assigns a start time so that peer-capacity constraints are never violated (i.e., a peer cannot send/receive more than its capacity allows), and all declared precedence relations in \(G_C\) are respected. Each transfer has a processing time \(T_{c}=\mathrm{size}(c)/\mathrm{rate}\), which we treat as a given positive integer after suitable scaling. The objective is to minimize the makespan \(C_{\max}\) of the warm-up; the \emph{decision version} asks whether there exists a feasible schedule with \(C_{\max}\le T^\star\). It is immediate that CSP is in NP: given a schedule (assignment of links and start times), one can verify in polynomial time that (i) every precedence constraint is respected, (ii) at all times each peer’s incident transmissions do not exceed its bandwidth (no overlap beyond capacity), and (iii) all chunks complete by \(T^\star\).

\subsection{NP-Hardness via \(P\mid\text{prec}\mid C_{\max}\)}
We reduce \(P\mid\text{prec}\mid C_{\max}\) to CSP by embedding identical-machine precedence-constrained scheduling as a special case of chunk scheduling over a star-like overlay (cf. \cite{Ullman1975}). Consider an instance with \(m\) identical machines, jobs \(J\), processing times \(\{p_j\}_{j\in J}\), precedence DAG \((J,\prec)\), and deadline \(T^\star\). Build \(G_P\) as a star with a central peer \(s\) and leaves \(v_1,\dots,v_m\). Calibrate capacities so that each leaf \(v_i\) receives at most one chunk at a time while different leaves can receive concurrently—mirroring \(m\) identical machines. For each job \(j\) create chunk \(c_j\) initially at \(s\) and required at some leaf; set \(T_{c_j}=p_j\). Sending \(c_j\) on \((s,v_i)\) simulates processing job \(j\) on machine \(i\). Encode precedence by zero-time \emph{unlock} relations that allow \(c_j\) to start at \(s\) only after all predecessors’ chunks have arrived at their leaves. Any CSP schedule with makespan \(\le T^\star\) corresponds one-to-one to a feasible \(P\mid\text{prec}\mid C_{\max}\) schedule (and conversely), establishing \(P\mid\text{prec}\mid C_{\max}\le_p\mathrm{CSP}\) and NP-hardness.

\subsection{Strong NP-Hardness via \textsc{3-Partition}}
For strong NP-hardness we reduce \textsc{3-Partition} \cite[pp.~96--101]{GareyJohnson1979} to CSP. Given integers \(A=\{a_1,\dots,a_{3m}\}\) with \(\sum_i a_i=mB\) and \(B/4<a_i<B/2\), it is NP-complete to decide whether \(A\) can be partitioned into \(m\) triples each summing to \(B\). Consider the special case of \(P\mid\text{prec}\mid C_{\max}\) with no precedences, \(m\) identical machines, and job lengths \(p_i=a_i\); a schedule of makespan \(\le B\) exists iff there is a perfect 3-partition (standard reduction; see \cite{GareyJohnson1979}). Applying the star construction above with chunks \(c_i\) of lengths \(T_{c_i}=a_i\) and deadline \(T^\star=B\) yields a CSP instance that is feasible iff the original \textsc{3-Partition} instance is a YES-instance. Because \textsc{3-Partition} is strongly NP-complete, CSP is strongly NP-hard under this encoding.

CSP belongs to NP and is NP-hard via \(P\mid\text{prec}\mid C_{\max}\); it is, moreover, strongly NP-hard via \textsc{3-Partition}. Consequently, optimizing warm-up chunk schedules in \emph{FLTorrent}—even under simplified star overlays and direct transfers—is computationally intractable in general. This extends to variants that additionally require each node to accumulate at least \(k\) chunks before warm-up ends: such constraints do not reduce complexity.
